# Supplementary material for: Quasi 1D electronic transport in a 2D magnetic semiconductor
Source: arXiv:2202.11427 ancillary file (2022-02-23)
Supplement: Supplementary file 1 [file CSB_resub.pdf]

# Supplementary Information for
# Quasi 1D electronic transport in a 2D magnetic semiconductor

Fan Wu,[1,2,*] Ignacio Gutiérrez-Lezama,[1,2] Sara A. Lopéz-Paz,[3] Marco Gibertini,[4] Kenji Watanabe,[5] Takashi Taniguchi,[6] Fabian O. von Rohr,[3] Nicolas Ubrig,[1,2,†] and Alberto F. Morpurgo[1,2,‡]

[1]*Department of Quantum Matter Physics, University of Geneva, 24 Quai Ernest Ansermet, CH-1211 Geneva, Switzerland*

[2]*Department of Applied Physics, University of Geneva, 24 Quai Ernest Ansermet, CH-1211 Geneva, Switzerland*

[3]*Department of Chemistry, University of Zurich, CH-8057 Zurich, Switzerland*

[4]*Dipartimento di Scienze Fisiche, Informatiche e Matematiche, University of Modena and Reggio Emilia, IT-41125 Modena, Italy*

[5]*Research Center for Functional Materials, National Institute for Materials Science, 1-1 Namiki, Tsukuba 305-0044, Japan*

[6]*International Center for Materials Nanoarchitectonics, National Institute for Materials Science, 1-1 Namiki, Tsukuba 305-0044, Japan*

## CONTENTS

S1. Methods 2
Crystal growth and characterization 2
Device fabrication 6
Transport measurements 7
Optical measurements 7

S2. First-principles calculations 8

S3. Additional magneto-transport data 9

S4. I-V characteristics of CrSBr multilayers 11

S5. Details of photocurrent measurements 13

S6. Density of states and joint density of states for a 1D wire 15

References 16

## S1. METHODS

### Crystal growth and characterization

CrSBr single crystals were grown by chemical vapor transport using elemental chromium (Alfa Aesar 99.99%) and freshly prepared disulfur bromide in a 7:13 molar ratio, as reported elsewhere [S1, S2]. The reactants were sealed under vacuum in a 20 cm length quartz ampule. After thermal treatment in a three-zone furnace with a temperature gradient of 950-880° C for 140 h, CrSBr crystals were isolated at the middle-cold end of the tube. The crystals were subsequently washed using warm pyridine, water and acetone. The needle-shaped black crystals were characterized by means of X-Ray diffraction (see Figure S1) using a STOE STADIP diffractometer in transmission geometry and a Rigaku SmartLab in reflection mode with Cu $K\alpha$ radiation. All the reflections are indexed within the *Pmmn* space group, in close

* fan.wu@unige.ch
† nicolas.ubrig@unige.ch
‡ alberto.morpurgo@unige.ch

correspondence with the reported structure for CrSBr [S2]. The chemical composition of the obtained CrSBr crystals was further checked by energy dispersive X-Ray spectroscopy (EDS) using a Zeiss GeminiSEM 450 scanning electron microscope equipped with EDX detectors. The elemental mapping (Figure S2) confirms the uniform distribution of the elements, with an atomic ratio Cr:S:Br of 32.8(3) : 32.4(2) : 34.8(2)) that is well in agreement with the expected 1:1:1 stoichiometry.

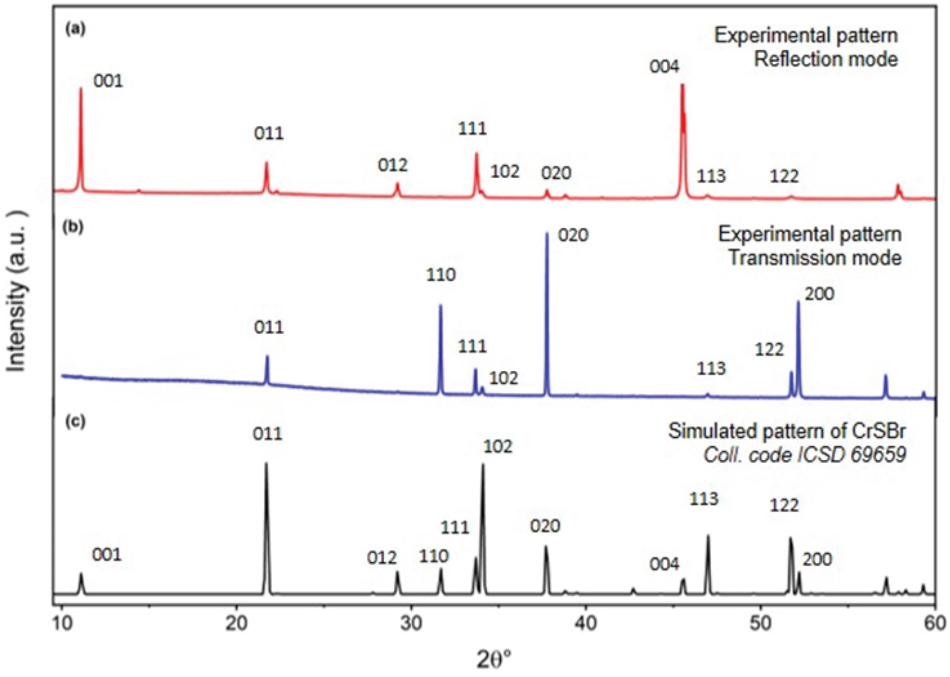


Figure S1. Experimental powder X-Ray diffraction (PXRD) patterns for CrSBr in (a) reflection and (b) transmission geometries, together with (c) the simulated PXRD pattern. The main reflections are indexed within the Pmmn space group. Due to the layered character of the structure, a strong preferential orientation is observed leading to an enhanced intensity for the {00l} and {hk0} reflections in reflection and transmission geometries, respectively.

We also characterized our CrSBr crystals by means of Raman spectroscopy. Raman spectra were acquired by illuminating thin crystals exfoliated onto a $SiO_2$/Si substrate with a 532 nm continuous wave laser (nominal power 60 $\mu$W), and collecting the scattered light with a microscope objective. The scattered light was fed into a spectrometer equipped with a $N_2$ cooled Si charge coupled device array (LabRAM HR Evolution), enabling a resolution

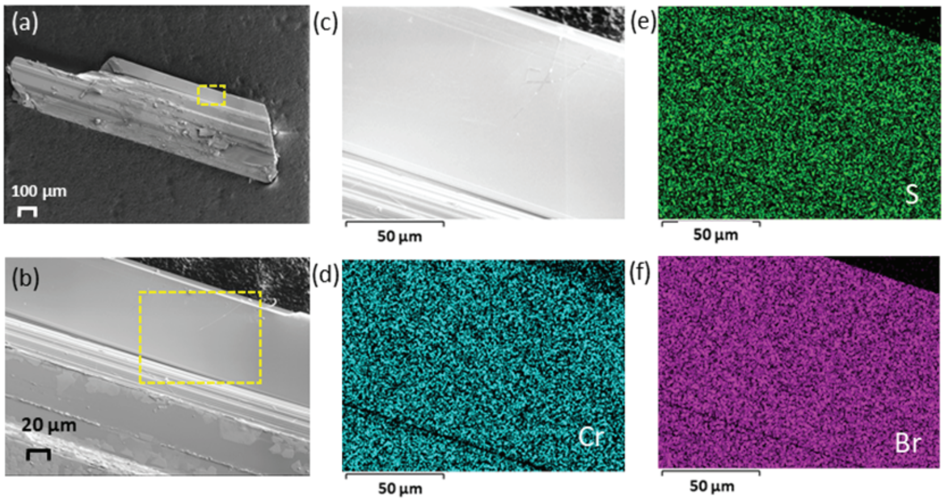


Figure S2. (a) SEM image of a CrSBr single crystal and (b-c) selected area for the EDS analysis. Elemental mapping for (d) Cr, (e) S and (f) Br, resulting in an atomic ratio Cr:S:Br of 32.8(3) : 32.4(2) : 34.8(2)).

of the optical spectra of 0.3 $cm^{-1}$. Figure S3 shows Raman peaks at 112, 244, and 343 $cm^{-1}$ for the 4 nm thick crystal shown in the inset, in good agreement with previously reported Raman measurements performed on few layers CrSBr [S3].

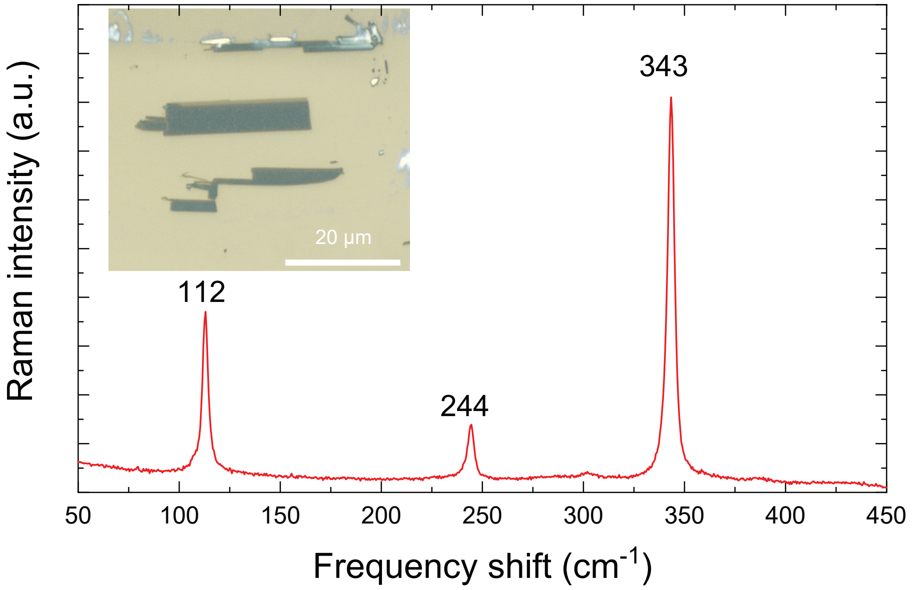


Figure S3. Raman spectrum of a 4 nm thin CrSBr multilayer (see optical microscopic image in the inset) freshly exfoliated on a $SiO_2$/Si substrate.

The magnetic properties of CrSBr as-grown single crystals have been assessed by means of DC magnetic susceptibility using a commercial *magnetic properties measurement system* (MPMS) superconducting quantum interference device (SQUID). The magnetic susceptibility (Figure S4) was measured as a function of temperature, with magnetic field applied perpendicular to the crystalline planes of the material. A peak in the susceptibility is observed at 132 K, in correspondence of the antiferromagnetic transition, in excellent agreement with previously reported results [S2, S4]. Upon further decreasing the temperature a small, reproducible kink is detected around 30 K (referred to as $T^*$), also consistent with earlier observations [S2, S4]. The kink results from a magnetic transition whose nature remains to be determined.

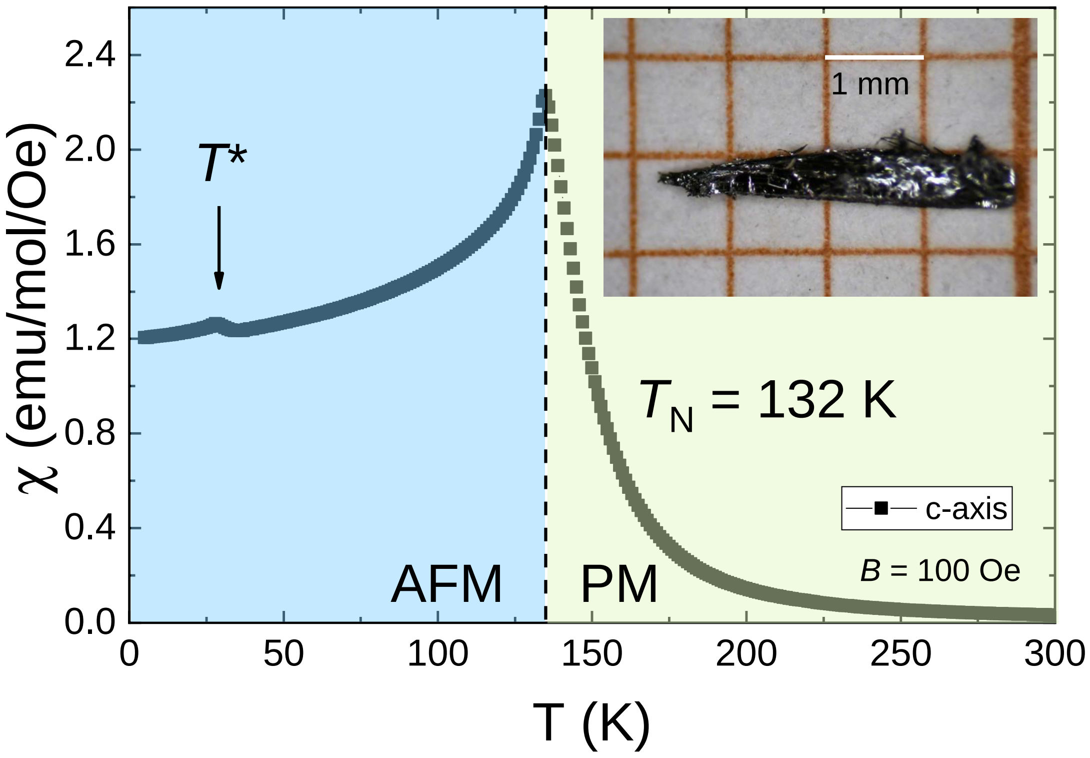


Figure S4. Temperature-dependent magnetic susceptibility of a bulk CrSBr single crystal, measured applying the magnetic field ($\mu_0 H = 0.01$ T) along the *c*-axis. The pronounced peak at 132 K determines the value of the *Néel* temperature $T_N$. Another kink is visible at 30 K, due to an additional magnetic transition, whose precise nature has yet to be identified. The inset shows an image of the crystal used for the susceptibility measurements.

## Device fabrication

CrSBr multilayers were obtained by exfoliating bulk crystals in a Nitrogen gas-filled glove box, with sub-ppm oxygen and water concentration to avoid possible degradation. The multilayer thickness was determined by means of atomic force microscopy, as shown in Figure S5. In some cases, the multilayers were encapsulated with exfoliated hBN layers, employing a conventional pick-up and release technique based on PC/PDMS polymer stacks placed on glass slides [S5] (as mentioned in the main text, CrSBr is significantly more stable than most other 2D magnetic materials and limited exposure to air does not appear to significantly affect its properties). A total of 14 devices have been fabricated and contacted with metallic electrodes (Pt/Au: 10/40 nm), using a conventional process based on electron-beam lithography, electron-beam evaporation, and lift-off (for hBN-encapsulated devices, the capping hBN layer in the contact area was removed by reactive ion etching with a $CF_4/O_2$ mixture prior to evaporation). Six devices have been intensively investigated as a function of temperature and magnetic field, showing the behavior that we discussed in the main text. On the other eight devices we performed exclusively room-temperature transport measurements, useful to increase the statistics of the in-plane conductivity values in both crystallographic directions.

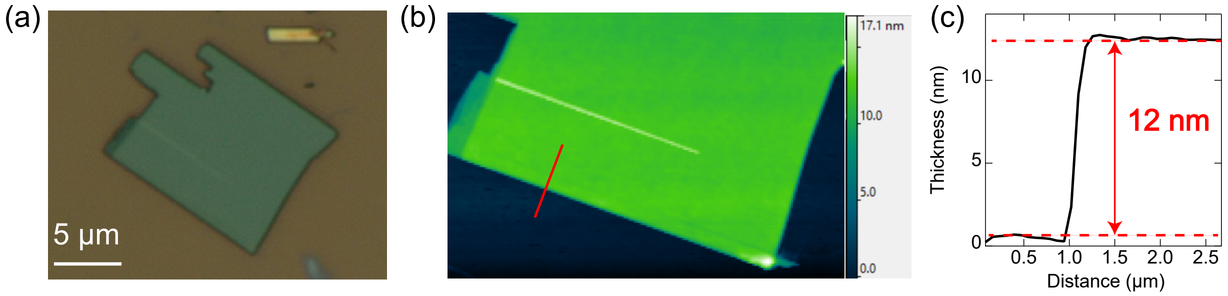


Figure S5. (a) Optical microscope and (b) atomic force microscope image of a CrSBr multilayer exfoliated on a silicon substrate. (c) Height profile measured along the red line in (b), allowing the thickness of the multilayer be determined.

### Transport measurements

Transport measurements were performed in a variable temperature insert of a cryogen-free Teaslatron cryostat (Oxford Instruments) equipped with a 12 T superconducting magnet. The electric-transport and magneto-transport properties were measured either in dc or with a low-frequency ac methods (using a Keithley 2400 source/measure unit and a SRS830 lock-in amplifier in combination with home-made low noise electronics).

### Optical measurements

Photoluminescence and photocurrent measurements were performed using a He-flow cryostat mounted under an optical microscope with optical access and electrical connections. All data presented in the main text or in the supplementary information were taken at $T = 10$ K. Photoluminescence measurements were performed in a backscattering geometry, with the same objective used to illuminate the sample and collect the re-emitted light. For these measurements, the laser wavelength was tuned to 633 nm and the power kept at 50 $\mu W$, with a diffraction limited beam size of about 1 $\mu$m. The incoming light was polarized linearly using a broadband *Glan-Taylor* polarizer, and the direction of the electric vector of light was adjusted with respect to the crystal axis by inserting a $\lambda/2$-plate in the optical path. The light collected from the sample was sent to a Czerny-Turner monochromator with a grating of 150 grooves/mm (Andor Shamrock 500i) and detected with a Silicon Charge Coupled Device (CCD) array (Andor Newton 970 EMCCD).

Photocurrent measurements were performed by illuminating the sample with a supercontinuum white light laser passing through a contrast filter, allowing the laser wavelength to be tuned continuously between 400 and 1100 nm, while keeping the power fixed at 100 $\mu$W. For these measurements, the sample was placed in the cryostat on a holder mounted on a piezo-electric driven $x - y$ stage, allowing stepping the position of the sample relative to the beam with a precision of 50 nm (Cryovac KONTI). The photocurrent was then measured with home-made low noise voltage and current amplifiers, and read out by digital multimeters.

## S2. FIRST-PRINCIPLES CALCULATIONS

First-principles calculations have been performed within density-functional theory by using the Quantum ESPRESSO suite of codes [S6, S7]. The Perdew-Burke-Ernzerhof (PBE) exchange-correlation functional [S8] has been adopted, with ultrasoft pseudopotentials from the GBRV library [S9] which give the best comparison with all electron calculations for the elements considered here [S10]. Converged results require an energy cutoff of 40 Ry to represent wave functions and 320 Ry for the charge density. The Brillouin zone is sampled using a $12 \times 9 \times 1$ $\Gamma$-centered Monkhorst-Pack grid. Artificial effects arising from the spurious periodic replicas along the vertical direction have been suppressed by using a cutoff on Coulomb interactions [S11]. Before performing band structure calculations, the atomic positions and unit cell parameters have been fully relaxed using a BFGS algorithm until the residual force on each atom was below 2.6 eV/Å and each component of stress below 0.5 kbar.

A result of our calculations is the band structure of monolayer CrSBr shown in Figure 1**b** of the main text, which exhibits a large anisotropy in the dispersion of the lowest conduction band (and of other bands). In order to gain some understanding for the origin of this strong anisotropy, in Figure S6 we report the orbital decomposition of the Bloch states as a function of crystal momentum along the $a$ and $b$ directions, corresponding respectively to $\Gamma$-X and $\Gamma$-Y in reciprocal space. Such decomposition is obtained by mapping the first-principles results for Bloch states around the energy gap into a set of maximally localized Wannier functions [S12] arising from Cr $d$-orbitals together with S and B $p$-orbitals, using the Wannier90 code [S13, S14]. Along $a$ (*i.e.*, $\Gamma$-X), there is a dominant ($> 80\%$) contribution from Cr $d$-orbitals, with a negligible weight from Br and S. The localized nature of $d$-states is responsible for a reduced hopping energy along this direction and thus to a very small band width. On the contrary, along $b$ (i.e. $\Gamma$-Y), there is a significant hybridization between Cr and S, which then gives rise to a much larger dispersion of the conduction band in this direction.

We emphasise that although this picture accounts for the strong band anisotropy found in first-principles results, it does not allow to determine on purely theoretical grounds what is the regime that is most appropriate to describe transport in CrSBr. Specifically, the result of the band structure calculations does not tell whether the transport properties are better

modelled in terms of a strongly anisotropic 2D electron system, or in terms of weakly and incoherently coupled 1D chains. The results of the experiments clearly indicate that –among the two–the second option is the most appropriate one.

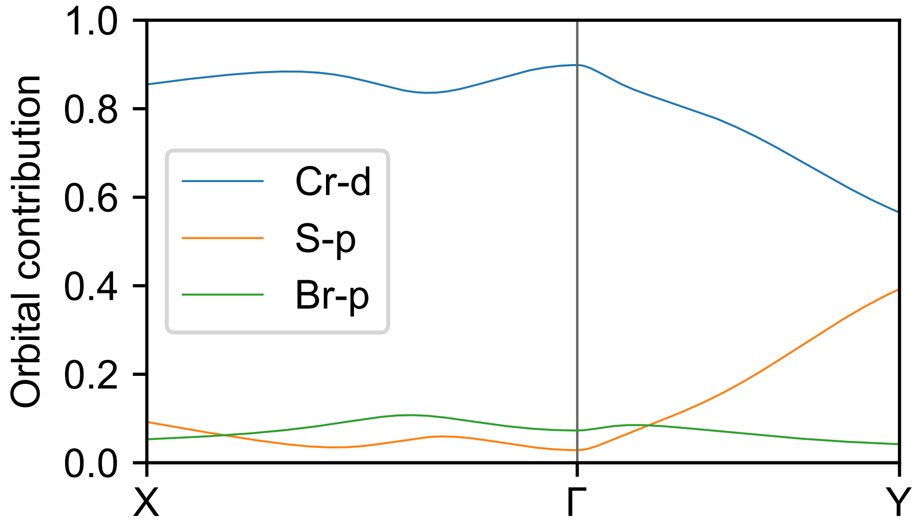


Figure S6. Orbital decomposition of the Bloch states corresponding to the lowest conduction band of monolayer CrSBr (see Fig. 1b in the main text), obtained by mapping the first-principles, density-functional theory results into a set of maximally localized Wannier functions [S12] (see Methods). The decomposition is shown along two directions in reciprocal space, Γ-X and Γ-Y, which correspond respectively to the $a$ and $b$ direction in real space.

## S3. ADDITIONAL MAGNETO-TRANSPORT DATA

In the main text, we have shown that magneto-resistance of CrSBr multilayers along the $a$ and $b$ crystallographic directions exhibit opposite sign when cooled down below 100 K. Here, we confirm that this effect is robust and reproducible, by showing, in Figure S7, the magnetic field dependence of the magneto-resistance ratio for two additional devices. The thickness of CrSBr in both devices is comparable, approximately 12 nm, and each individual device probes the magneto-transport either along the $a$ or the $b$ crystallographic direction (see Figures S7 (a) and (b), respectively). Consistently with what we have shown in the main text, the low-temperature magneto-resistance is negative when the current passes along the

$a$ crystallographic direction and positive in the $b$ crystallographic direction.

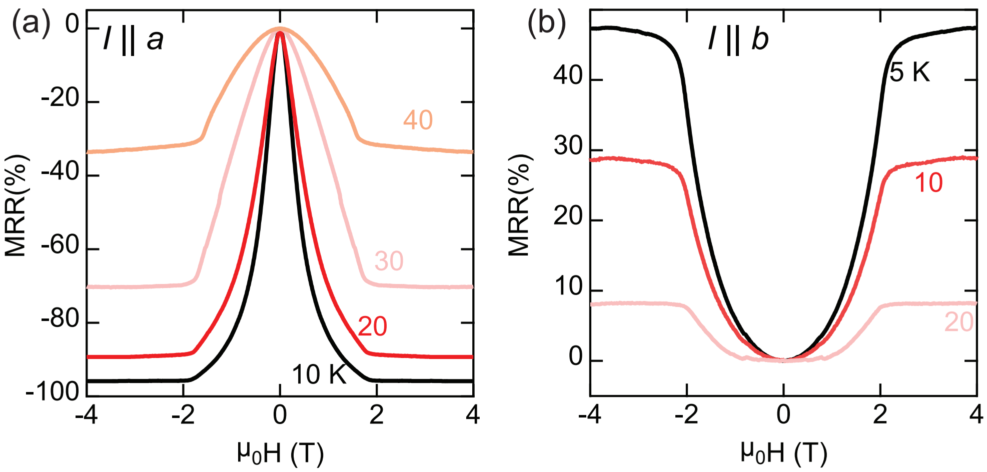


Figure S7. Longitudinal magnetoresistance ratio (MRR $= (R(\mu_0 H) - R(0))/R(0)$) measured on two distinct 12 nm thick CrSBr devices with current flowing in the (a) $a$-direction and the (b) $b$-direction respectively. The different curves represent measurements done at different temperatures as indicated in the figures. The magnetic field is applied along the $c$ crystallographic direction in both cases.

A clear indication that the electronic transport in CrSBr is incompatible with 2D band-like transport, is the absence of a measurable Hall effect in all samples that we have investigated. As we have mentioned in the main manuscript, irrespective of their thicknesses, crystallographic direction along which the current flows, temperature, and gate voltage the transverse voltage that we measure is symmetric in the applied magnetic field. In Figure 4 of the main text we illustrate this with data measured on two devices.

To further substantiate our statement, we present in Figure S8 data from additional devices on which we have tried to measure the Hall effect. In agreement with the samples presented in the main text, the transverse resistance remains symmetric with the applied magnetic field irrespective of temperature (Figure S8 (a)) or gate voltage (Figure S8 (b)). In particular Figure S8 (a) shows that the transverse resistance is symmetric both when the temperature $T$ is larger or smaller than $T_N$. Cooling down across the Néel temperature does not lead to any qualitative new feature in the transverse resistance. At lower temperature the longitudinal resistance increases and the transverse resistance does the same, supporting the idea that what is detected in the measurements of transverse resistance as a function of

magnetic field is *de facto* a component of longitudinal magnetoresistance. Indeed, also the gate voltage dependence of the transverse resistance is consistent with this idea: the application of a larger positive gate voltage decreases the longitudinal resistance and similarly a decrease is observed in the transverse resistance (see Figure S8 (b)).

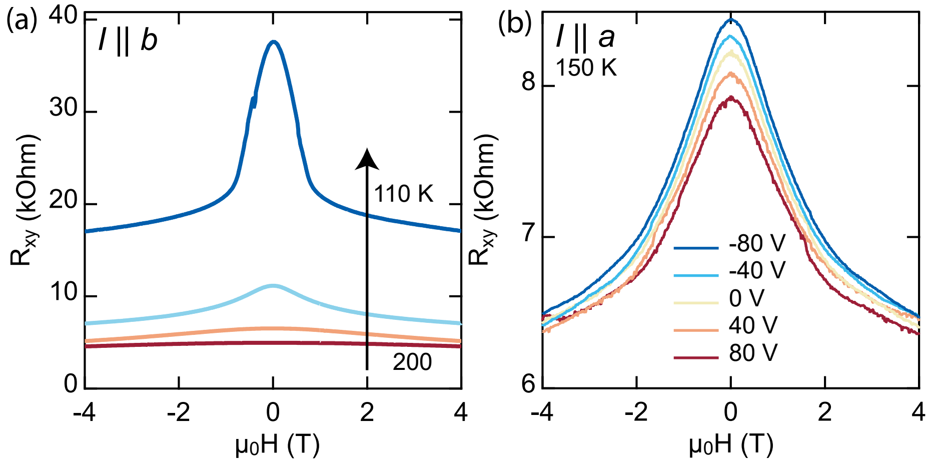


Figure S8. (a) Transverse magnetoresistance of a 5 nm thick CrSBr device with current flowing along $b$-direction measured from 110 to 200 K every 30 K, as the temperature is varied across the Nèel temperature $T_N = 132$ K . (b) Transverse magnetoresistance of a 6 nm CrSBr device with current flowing along $a$-direction at 150 K with different values of applied gate voltage $V_G$ (from -80 V to 80 in 40 V steps). The magnetic field is applied perpendicular to the CrSBr layers in both cases.

## S4. I-V CHARACTERISTICS OF CrSBr MULTILAYERS

In the main text we have discussed the longitudinal and transverse the conductivity $\sigma_a$ and $\sigma_b$ in the $a$ and $b$ crystallographic directions as a function of temperature, gate voltage, and magnetic field, i.e., the linear transport properties of CrSBr. For completeness –as it may be relevant in the context of 1D transport– here we show the full $I-V$ characteristics measured in the two directions, with applied bias that is sufficiently large to enter the non-linear regime.

$I-V$ characteristics measured at $T = 5$ K in the in the $a$- and $b$-direction are plotted in Figures S9**a**,**b** respectively, with the data showing a pronounced non-linearity. Measure-

ments are performed in a four-terminal configuration to ensure that the non-linearity is not generated by the contact resistance (indeed, metal/semiconductor contacts commonly exhibit non-linear $I-V$ characteristics). Figures S9**c** shows the same $I-V$ characteristics plotted in a double-logarithmic scale, which makes apparent different aspects of the data. First, as expected, for the same applied bias the current along the $b$-direction is several orders of magnitude larger than along the $a$-direction. Second, the $I-V$ curves in both directions exhibit different regimes, in which the relation between $log(I)$ and $log(V)$ is approximately linear, i.e., in which the $I-V$ characteristics are power-law like. For both directions, the slope (which corresponds to the exponent of the power law relation) is 1 at low bias, as it should be (since at sufficiently low applied voltage as compared to $k_BT$ –where $k_B$ is the Boltzmann constant– the $I-V$ characteristics are always linear). At larger bias the slope increases for both directions. In the the $a$-direction the slope at higher bias is approximately 2.5; in the $b$-direction, an interval with slope 3.5 is followed by a high bias regime with a slope that is approximately 2. In all cases in which we measured the $I-V$ characteristics of the devices up to sufficiently high bias a qualitatively similar power-law-like non-linearity has been observed, but based on our statistics we cannot confirm that the values of the exponents in the different regimes are always the same (i.e., the same in different devices).

Whereas it is certainly relevant to show the non-linear behavior of the $I-V$ curves – because different transport mechanisms peculiar of 1D conductors (both for transport along the conductor and for tunneling into it) may result in a power law $I-V$ curves similar to the ones we observe– we emphasize that rather mundane mechanisms (such as, for instance, space-charge limited current) may be at the origin of the observed behavior [S15–S17].

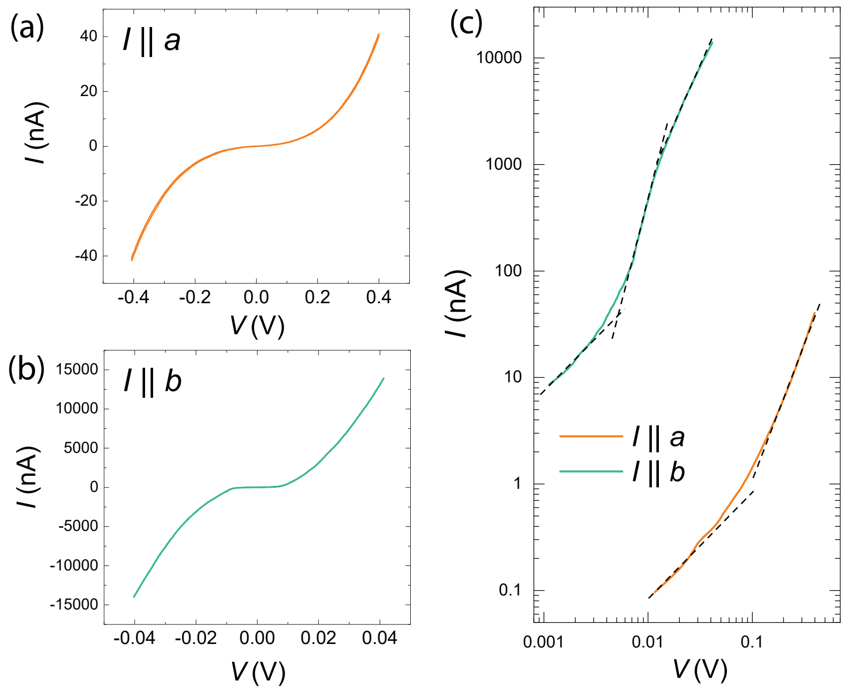


Figure S9. (a),(b) $I-V$ characteristics of CrSBr multilayers measured in a four-terminal configuration, for current flowing respectively along the $a$ or the $b$ crystallographic direction. (c) Same data as in panel (a) and (b) plotted in double logarithmic scale, showing that the non-linearity of the $I-V$ curves exhibits a power-law like behavior. The black dashed line represents linear fitting in different bias regime, and allow extracting the exponent of the power law relation. In the $a$-direction the exponent changes from 1 at low bias to approximately 2.5 at higher bias; in the $b$-direction the exponent changes from 1 at low bias to approximately 2 at high bias, with an intermediate region exhibit an exponent of 3.5. All data are measured at $T = 5$ K.

## S5. DETAILS OF PHOTOCURRENT MEASUREMENTS

In the main text, we have shown the spectral dependence of the photocurrent measured in CrSBr multilayer devices, which is naturally interpreted in terms of a van Hove singularity characteristic of a 1D band. Here, we discuss the experimental details of the photocurrent measurements.

Photocurrent is measured directly connecting together source and drain contacts, in the absence of any applied bias, upon raster-scanning a laser spot ($\approx 2$ $\mu$m in diameter) over the

surface of the CrSBr multilayer (see Figure S10 (a) and (b)). The result of the measurement provides us with a map of the photocurrent intensity as a function of laser spot position (see Figure S10 (c) and (d); data taken at laser wavelength $\lambda = 910$ nm). As it is typical in photocurrent measurements on a gapped semiconductors at zero applied bias, a finite photocurrent signal is only observed if the light wavelength corresponds to an energy at least equal to the (optical) gap, and if the laser spot is sufficiently close to one of the contacts (see Figure S10 (b)). Additionally, the sign of the photocurrent changes upon moving the laser spot from one contact to the other (see Figure S10 (d)). The microscopic process responsible for this behavior is common to all semiconductors: the minority carrier of the photoexcited electron-hole pairs (holes, in the case of CrSBr multilayers) escapes through the nearby contact, resulting in the measured current. This mechanism naturally explains why the current reverts its sign if the laser spot is shifted from one contact to the other (simply because the holes escape through different contacts in the two cases) and why it vanishes if the laser spot is far away from either contact (because the photoexcited electron and hole pairs recombine before the minority carrier can escape at a contact).

At any given energy of the incident photons, the magnitude of the photocurrent is determined by the amount of minority carriers –determined by the absorption rate of photons at that energy energy $E = h\nu$– that are eventually extracted at the contact (as discussed above). The dependence of the photocurrent on the energy of the incoming photon is a measure of the absorption spectrum of the material and, in the simplest possible scenario, it is determined by its joint density of states. Indeed, the spectral and polarization dependence of the photocurrent is the same irrespective of where the laser spot is positioned, which confirms that the experiment probes the ability of the material to absorb light at a given energy (the photocurrent spectra shown in the main text are acquired with the spot positioned near one of the contacts, where current intensity is the highest, and the signal-to-noise ratio is optimal). Indeed, using photocurrent measurements to probe the absorption spectrum of semiconductors and of their heterostructures is a technique that has been employed already long ago [S18, S19] to investigate III-V heterostructures. As compared to direct absorption measurements, it has multiple technical advantages. Possibly the most important one is to avoid working with transparent substrates –as it would be needed to measure absorption in a transmission experiment– which would make device fabrication much more complex (or even impossible in some cases).

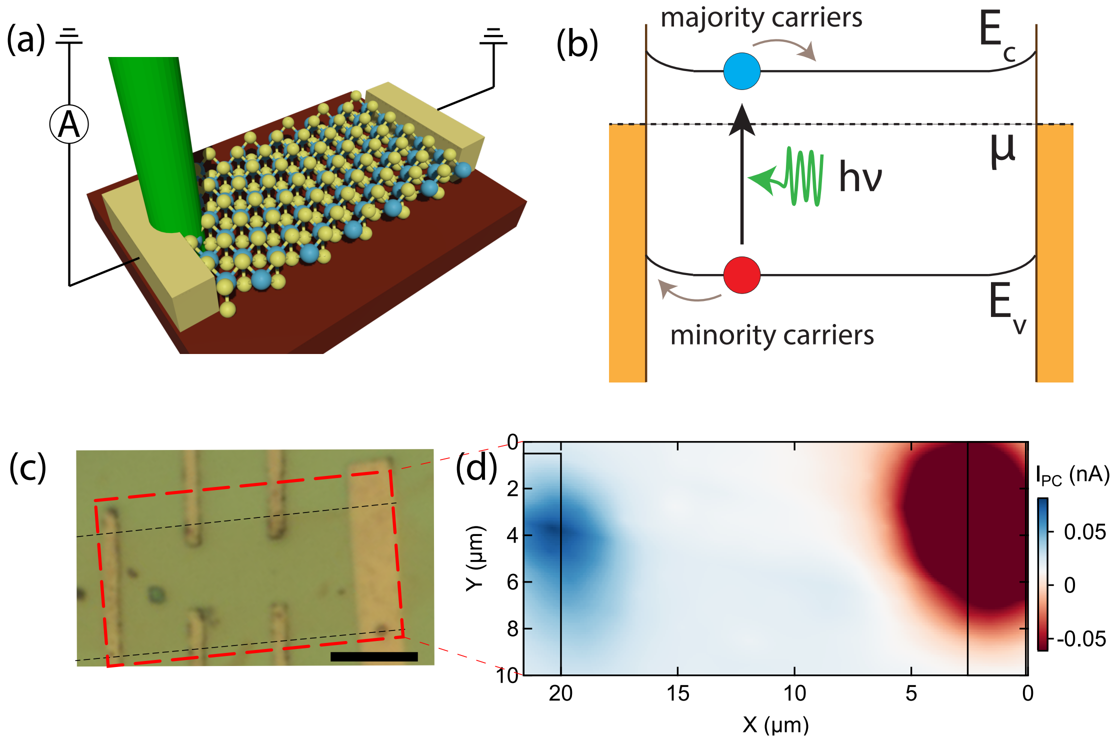


Figure S10. (a) Schematics of the experimental configuration in which photocurrent measurements are performed. The photocurrent is measured upon illuminating the sample, after having short circuited the source and drain contacts. (b) Illustration of the band diagram for an electron-doped semiconductor, showing band bending at the metal/semiconductor contacts. The measured photocurrent results from the escape of photogenerated minority carriers (in the present case holes represented by the red circle) from the semiconductor into the nearby metal contact. (c) Optical microscope image of a device used for the photocurrent measurements. The scale bar represents 5 $\mu$m. The black dashed line outlines the limits of the CrSBr multilayer. The red dashed line delimits the area which is raster-scanned by the laser to obtain the spatial dependence of the photocurrent shown in (d). The thin black lines in (d) indicate the position of the edges of the metallic contacts used in the measurements.

## S6. DENSITY OF STATES AND JOINT DENSITY OF STATES FOR A 1D WIRE

In the main text, we have shown that electronic states in CrSBr have a 1D character and we have argued based on experimental evidence that the electronic properties are better captured by modeling the material as a collection of weakly coupled 1D wires, than by viewing it as an anisotropic 2D electronic system. Here we show that modeling the material

as a collection of 1D wires allows us to easily understand why the joint density of states (JDOS) probed by photocurrent measurements [S20] gives rise to a singularity close to the onset for interband transitions, which has the same energy dependence as the *van Hove* singularity in the density of states of 1D bands.

Modeling CrSBr as a collection of 1D wires implies that –for the dispersion of the conduction and valence band close to the band edges– we can write $E_v(k) = E_v - \hbar^2 k^2/(2m_v^*)$ and $E_c(k) = E_c + \hbar^2 k^2/(2m_c^*)$ (for the valence and conduction band respectively; here $m_{c,v}^* > 0$ are the respective effective masses and $E_{c,v}$ are the band extrema, so that $E^* = E_c - E_v$ is the energy gap). The JDOS at energy $E$ is defined as the number of interband transition energies $E_c(k) - E_v(k)$ (per unit length) between $E$ and $E + dE$, with $dE$ infinitesimal, and it is thus given by

$$J(E) = \int \delta\left(E - E_c(k) + E_v(k)\right) \frac{dk}{2\pi} = \int \delta\left(E - E^* - \frac{\hbar^2 k^2}{2m_c^*} - \frac{\hbar^2 k^2}{2m_v^*}\right) \frac{dk}{2\pi} \tag{1}$$

By introducing the (inverse) reduced mass $1/m^* = 1/m_c^* + 1/m_v^*$, we thus have that

$$J(E) = \int \delta\left(E - E^* - \frac{\hbar^2 k^2}{2m^*}\right) \frac{dk}{2\pi} \tag{2}$$

which is equivalent to the density of states of a single band with dispersion $E_n(k) = E^* + \hbar^2 k^2/(2m^*)$. In particular, close to the onset for interband transitions ($E \simeq E^*$) we have [S20]

$$J(E) = \frac{1}{2\pi\hbar}\sqrt{\frac{2m^*}{E - E^*}} \propto 1/\sqrt{E - E^*} \tag{3}$$

which is the $1/\sqrt{E - E^*}$ mentioned in the main text.

We conclude noting that, within a 1D model, a similar $1/\sqrt{E - E^*}$ would be obtained also considering a transition between a localized defect state (acting as “valence band”), $E_v(k) = E_0$, and the 1D conduction state, in which case the reduced mass coincides with the conduction band effective mass, $m^* = m_c^*$.

---


[S1] J. Beck, *Zeitschrift für anorganische und allgemeine Chemie* **1990**, *585*, 1 157.

[S2] E. J. Telford, A. H. Dismukes, K. Lee, M. Cheng, A. Wieteska, A. K. Bartholomew, Y. Chen, X. Xu, A. N. Pasupathy, X. Zhu, C. R. Dean, X. Roy, *Advanced Materials* **2020**, *32*, 37 2003240.

[S3] K. Lee, A. H. Dismukes, E. J. Telford, R. A. Wiscons, J. Wang, X. Xu, C. Nuckolls, C. R. Dean, X. Roy, X. Zhu, *Nano Letters* **2021**, *21*, 8 3511.

[S4] E. J. Telford, A. H. Dismukes, R. L. Dudley, R. A. Wiscons, K. Lee, J. Yu, S. Shabani, A. Scheie, K. Watanabe, T. Taniguchi, D. Xiao, A. N. Pasupathy, C. Nuckolls, Z. Xiaoyang, C. R. Dean, X. Roy, *arXiv preprint arXiv:2106.08471* **2021**.

[S5] L. Wang, I. Meric, P. Y. Huang, Q. Gao, Y. Gao, H. Tran, T. Taniguchi, K. Watanabe, L. M. Campos, D. A. Muller, J. Guo, P. Kim, J. Hone, K. L. Shepard, C. R. Dean, *Science* **2013**, *342*, 6158 614.

[S6] P. Giannozzi, S. Baroni, N. Bonini, M. Calandra, R. Car, C. Cavazzoni, Davide Ceresoli, G. L. Chiarotti, M. Cococcioni, I. Dabo, A. D. Corso, S. d. Gironcoli, S. Fabris, G. Fratesi, R. Gebauer, U. Gerstmann, C. Gougoussis, Anton Kokalj, M. Lazzeri, L. Martin-Samos, N. Marzari, F. Mauri, R. Mazzarello, Stefano Paolini, A. Pasquarello, L. Paulatto, C. Sbraccia, S. Scandolo, G. Sclauzero, A. P. Seitsonen, A. Smogunov, P. Umari, R. M. Wentzcovitch, *Journal of Physics: Condensed Matter* **2009**, *21*, 39 395502.

[S7] P. Giannozzi, O. Andreussi, T. Brumme, O. Bunau, M. Buongiorno Nardelli, M. Calandra, R. Car, C. Cavazzoni, D. Ceresoli, M. Cococcioni, N. Colonna, I. Carnimeo, A. Dal Corso, S. De Gironcoli, P. Delugas, R. A. Distasio, A. Ferretti, A. Floris, G. Fratesi, G. Fugallo, R. Gebauer, U. Gerstmann, F. Giustino, T. Gorni, J. Jia, M. Kawamura, H. Y. Ko, A. Kokalj, E. Kücükbenli, M. Lazzeri, M. Marsili, N. Marzari, F. Mauri, N. L. Nguyen, H. V. Nguyen, A. Otero-De-La-Roza, L. Paulatto, S. Poncé, D. Rocca, R. Sabatini, B. Santra, M. Schlipf, A. P. Seitsonen, A. Smogunov, I. Timrov, T. Thonhauser, P. Umari, N. Vast, X. Wu, S. Baroni, *Journal of Physics Condensed Matter* **2017**, *29*, 46 465901.

[S8] J. P. Perdew, K. Burke, M. Ernzerhof, *Physical Review Letters* **1996**, *77*, 18 3865.

[S9] K. F. Garrity, J. W. Bennett, K. M. Rabe, D. Vanderbilt, *Computational Materials Science* **2014**, *81* 446.

[S10] G. Prandini, A. Marrazzo, I. E. Castelli, N. Mounet, N. Marzari, *npj Computational Materials* **2018**, *4*, 1 72.

[S11] T. Sohier, M. Calandra, F. Mauri, *Phys. Rev. B* **2017**, *96*, 7 075448.

[S12] N. Marzari, A. A. Mostofi, J. R. Yates, I. Souza, D. Vanderbilt, *Rev. Mod. Phys.* **2012**, *84* 1419.

[S13] A. A. Mostofi, J. R. Yates, G. Pizzi, Y.-S. Lee, I. Souza, D. Vanderbilt, N. Marzari, *Computer*

*Physics Communications* **2014**, *185*, 8 2309.

[S14] G. Pizzi, V. Vitale, R. Arita, S. Blügel, F. Freimuth, G. Géranton, M. Gibertini, D. Gresch, C. Johnson, T. Koretsune, J. Ibañez-Azpiroz, H. Lee, J.-M. Lihm, D. Marchand, A. Marrazzo, Y. Mokrousov, J. I. Mustafa, Y. Nohara, Y. Nomura, L. Paulatto, S. Poncé, T. Ponweiser, J. Qiao, F. Thöle, S. S. Tsirkin, M. Wierzbowska, N. Marzari, D. Vanderbilt, I. Souza, A. A. Mostofi, J. R. Yates, *Journal of Physics: Condensed Matter* **2020**, *32*, 16 165902.

[S15] A. Rose, *Phys. Rev.* **1955**, *97* 1538.

[S16] M. A. Lampert, P. Mark, *Current injection in solids*, Academic press, **1970**.

[S17] Y. B. Zhu, L. K. Ang, *Journal of Applied Physics* **2011**, *110*, 9 094514.

[S18] D. A. B. Miller, D. S. Chemla, T. C. Damen, A. C. Gossard, W. Wiegmann, T. H. Wood, C. A. Burrus, *Physical Review B* **1985**, *32*, 2 1043.

[S19] R. T. Collins, K. v. Klitzing, K. Ploog, *Physical Review B* **1986**, *33*, 6 4378.

[S20] G. Grosso, G. Parravicini, *Solid State Physics*, Elsevier Science, **2013**.
